# Supplementary material for: State-of-the-art electroweak Higgs boson pair production in association with two jets at the LHC in the Standard Model and beyond
Source: arXiv:2511.02488 source file (2025-11-04)

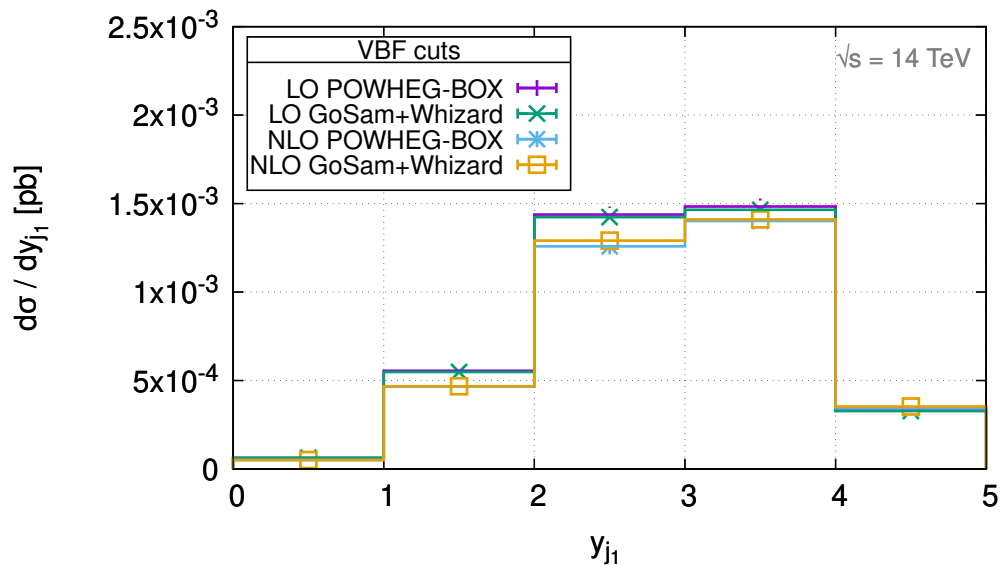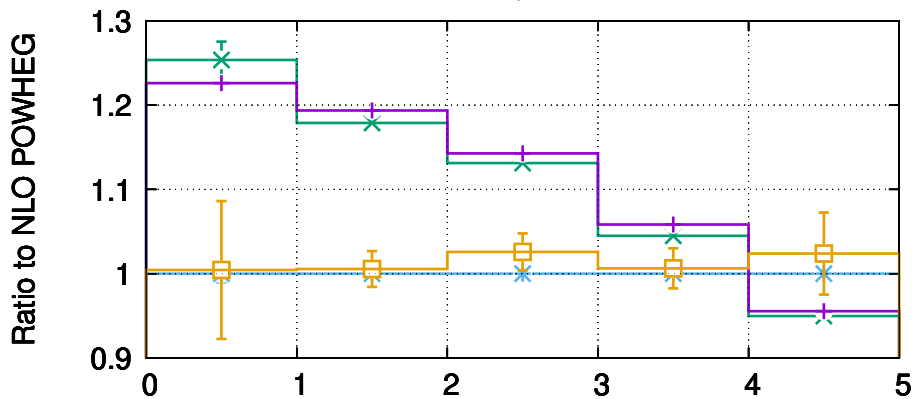

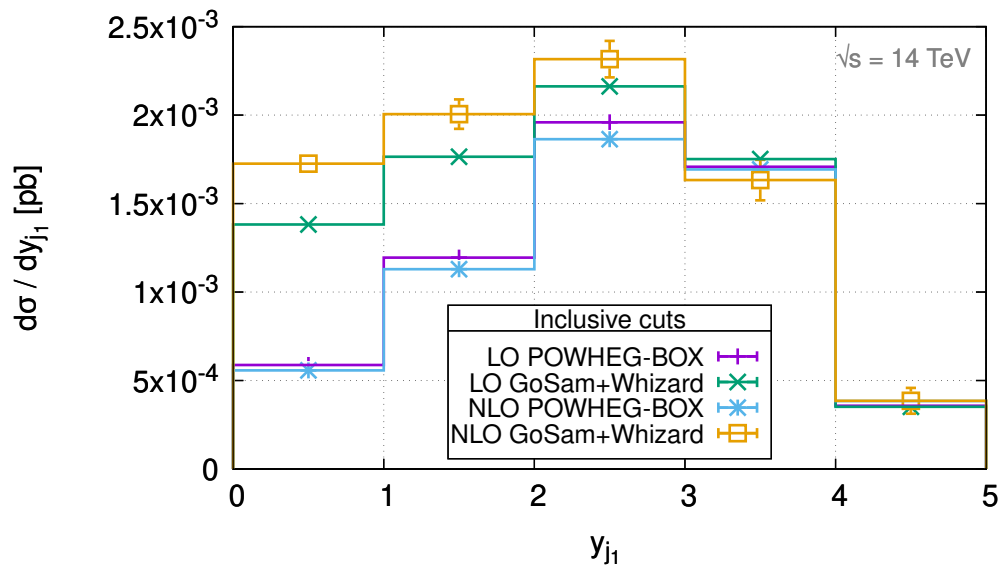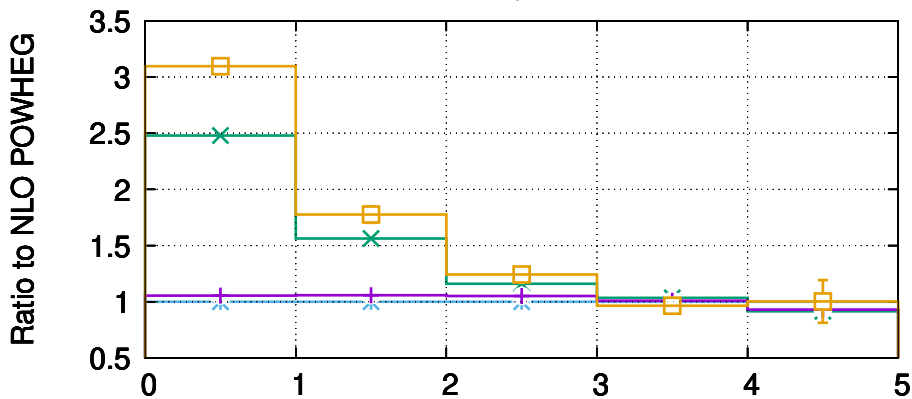



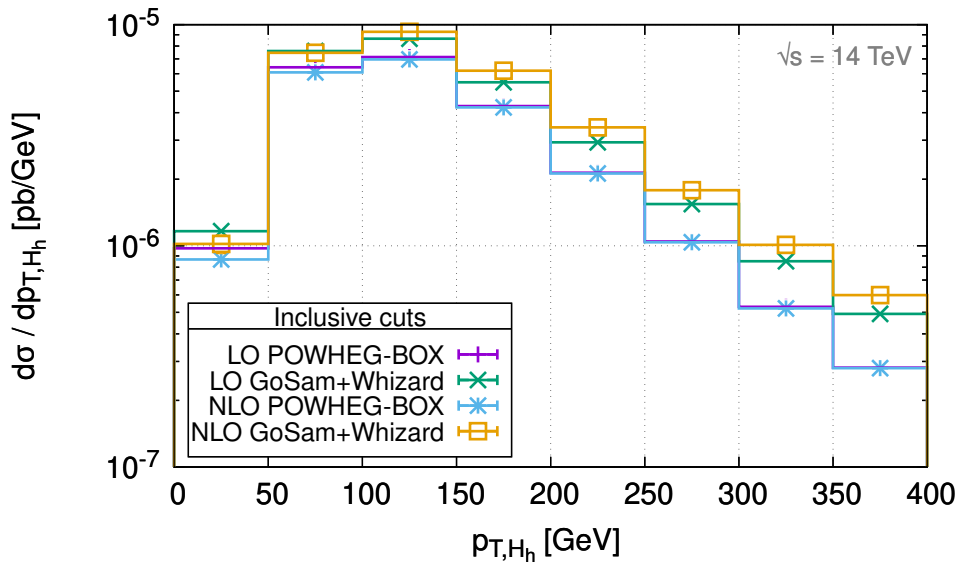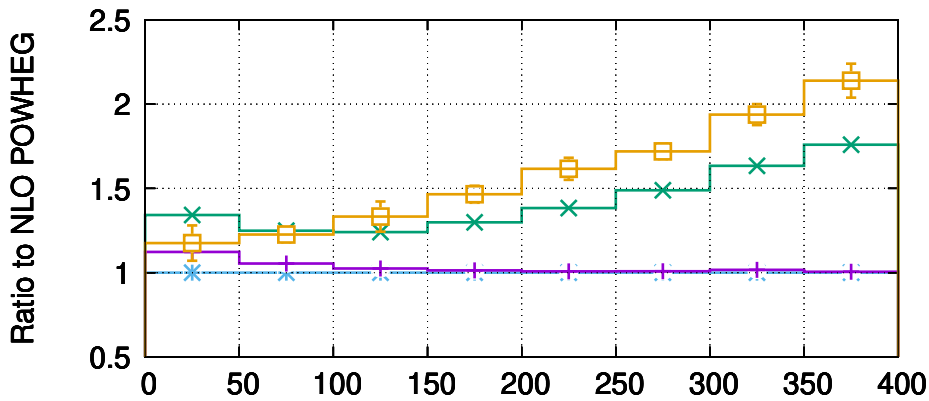

Supplement: Supplementary file 1 [file Plots-SM_s.pdf]
